# Supplementary material for: SumQE: a BERT-based Summary Quality Estimation Model
Source: arXiv:1909.00578 ancillary file (2019-09-02)
Supplement: Supplementary file 1 [file SumQE_Supplementary_Material.pdf]

# SUM-QE: a BERT-based Summary Quality Estimation Model Supplementary Material

**Stratos Xenouleas**[1], **Prodromos Malakasiotis**[1],
**Marianna Apidianaki**[2] and **Ion Androutsopoulos**[1]
[1] Department of Informatics, Athens University of Economics and Business, Greece
[2] CNRS, LLF, France and University of Helsinki, Finland
stratosxen@gmail.com, rulller@aueb.gr
marianna.apidianaki@helsinki.fi, ion@aueb.gr

## 1 Correlation between Linguistic Quality Criteria

Figures 2, 3 and 4 show correlation heatmaps between the five linguistic quality criteria in Figure 1. Correlation is calculated using Spearman's $\rho$, Kendall's $\tau$ and Pearson's $r$, and the scores manually assigned to summaries for each $\mathcal{Q}$ in the DUC-05, DUC-06 and DUC-07 datasets (Dang, 2006a,b; Over et al., 2007).

We observe that $\mathcal{Q}3$, $\mathcal{Q}4$ and $\mathcal{Q}5$ are highly correlated, which is unsurprising since a well structured and coherent summary should also use clear referential expressions, and preserve the focus. Driven by this observation, we used a pre-trained BERT model (BERT-FR-NS) to calculate the sentence perplexity as described in the main paper.

> **$\mathcal{Q}1$ – Grammaticality:** The summary should have no datelines, system-internal formatting, capitalization errors or obviously ungrammatical sentences (e.g., fragments, missing components) that make the text difficult to read.
>
> **$\mathcal{Q}2$ – Non redundancy:** There should be no unnecessary repetition in the summary.
>
> **$\mathcal{Q}3$ – Referential Clarity:** It should be easy to identify who or what the pronouns and noun phrases in the summary are referring to.
>
> **$\mathcal{Q}4$ – Focus:** The summary should have a focus; sentences should only contain information that is related to the rest of the summary.
>
> **$\mathcal{Q}5$ – Structure & Coherence:** The summary should be well-structured and well-organized. The summary should not just be a heap of related information, but should build from sentence to sentence to a coherent body of information about a topic.

Figure 1: Sum-QE rates the automatic summaries with respect to these five linguistic quality criteria. The datasets we use for tuning and evaluation contain human assigned scores (from 1 to 5) for each of these categories.

## 2 Selecting the Optimal Number of BPEs for GPT-2 and BERT-FR-LM

As explained in Section 4.2 of the article, a reasonable estimation of the $\mathcal{Q}1$ (Grammaticality) score is the perplexity returned by a pre-trained language model. We compare the performance of the fine-tuned BERT models for $\mathcal{Q}1$ to that of GPT-2 (Radford et al., 2019) and to the probability estimates that BERT with frozen parameters (FR) can produce for each token, treating it as a masked token (BERT-FR-LM). Both models use byte pair encodings (BPEs) as tokens.

Since perplexity tends to favor short texts and the grammaticality of a summary can be corrupted by only a few mistakes, we can focus on these mistakes and calculate the perplexity on the $k$ BPEs with the lowest probability. Figures 5, 6 and 7 show the correlations of GPT-2 for different values of $k$ (number of worst BPEs) on DUC-05, DUC-06 and DUC-07, respectively. Note that the optimal value of $k$ varies significantly across datasets making the use of LMs impractical for QE. The same conclusions hold for BERT-FR-LM (Figures 8, 9 and 10).

## 3 Summary Scoring Example

In Figure 11, we present an example of a high quality system summary from the DUC-07 dataset. Table 1 shows the scores assigned to that summary by the BERT and BiGRU-based SUM-QE models that had the best performance for each particular $\mathcal{Q}$. BERT makes more accurate estimations than BiGRU-ATT for all but one quality scores. Notably, the estimations for $\mathcal{Q}1$, $\mathcal{Q}2$ and $\mathcal{Q}4$ are very close to the gold scores.

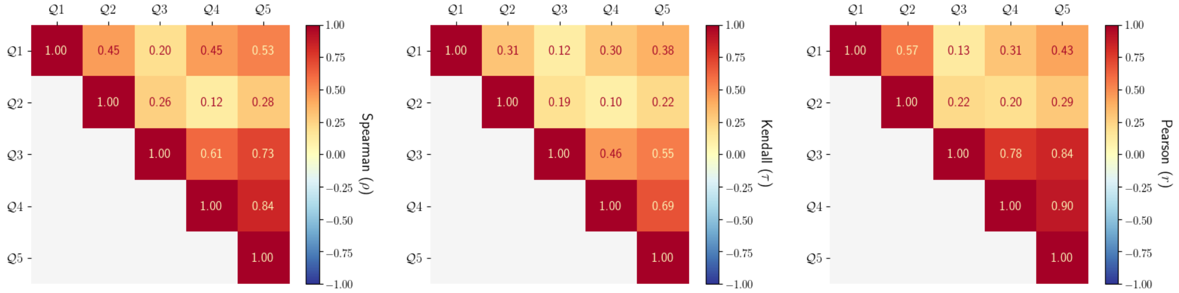


Figure 2: Spearman's $\rho$, Kendall's $\tau$ and Pearson's $r$ correlation heatmaps between the five $Q$s for DUC-05.

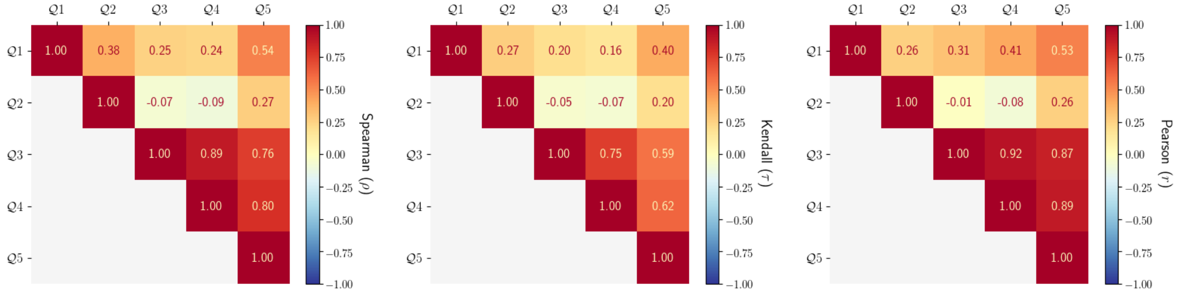


Figure 3: Spearman's $\rho$, Kendall's $\tau$ and Pearson's $r$ correlation heatmaps between the five $Q$s for DUC-06.

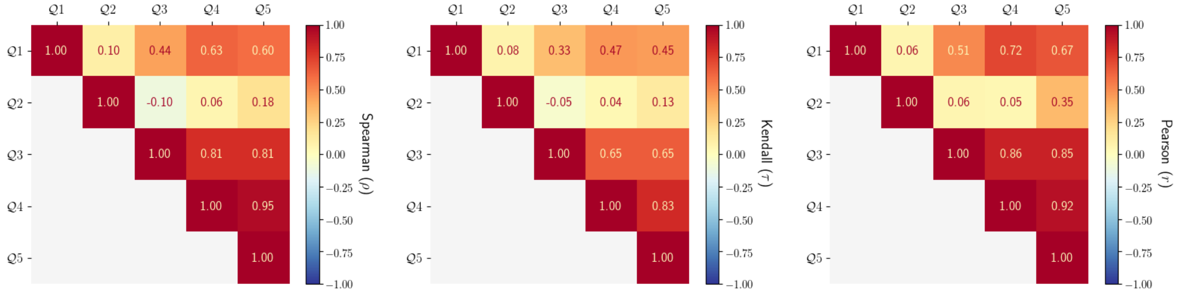


Figure 4: Spearman's $\rho$, Kendall's $\tau$ and Pearson's $r$ correlation heatmaps between the five $Q$s for DUC-07.

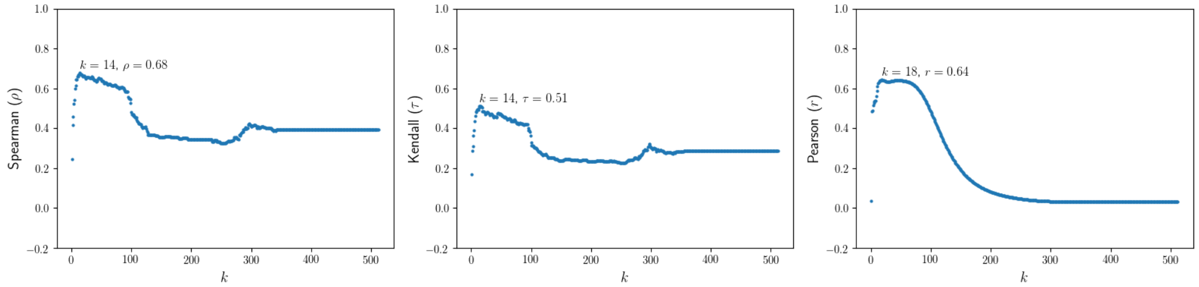


Figure 5: Spearman's $\rho$, Kendall's $\tau$ and Pearson's $r$ correlations for GPT-2 with each $k$ on DUC-05.

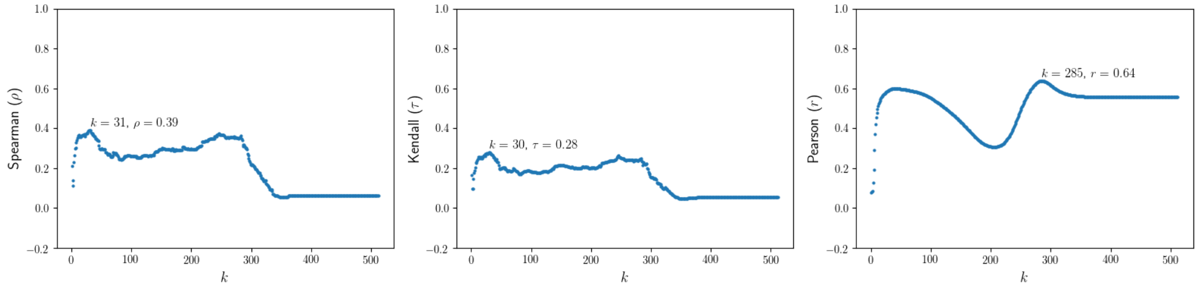


Figure 6: Spearman's $\rho$, Kendall's $\tau$ and Pearson's $r$ correlations for GPT-2 with each $k$ on DUC-06.

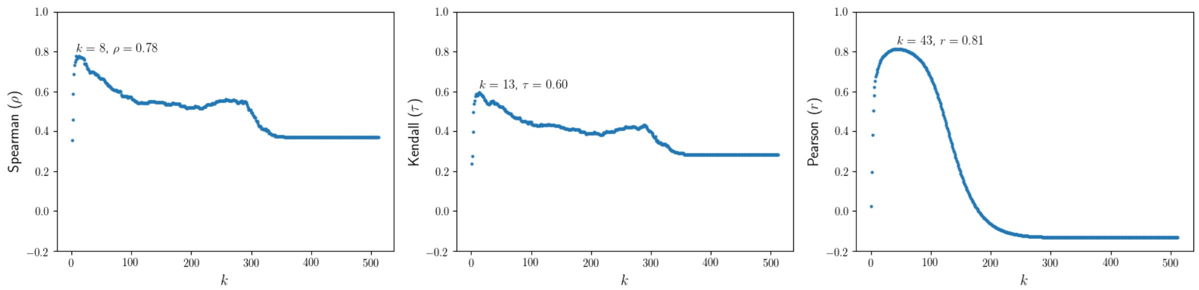


Figure 7: Spearman's $\rho$, Kendall's $\tau$ and Pearson's $r$ correlations for GPT-2 with each $k$ on DUC-07.

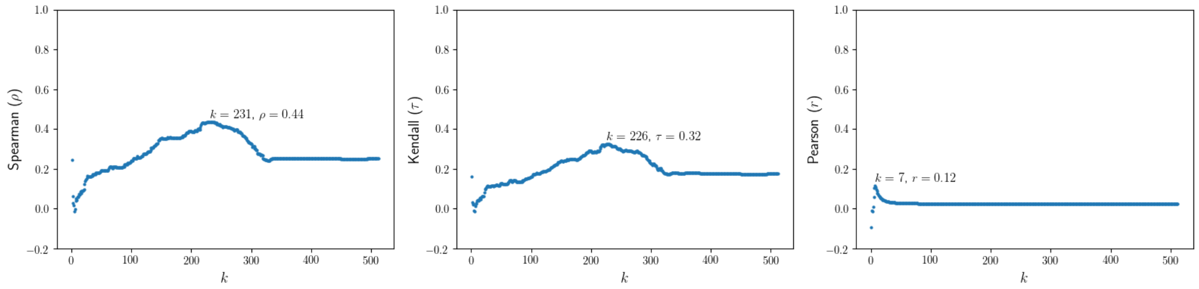


Figure 8: Spearman's $\rho$, Kendall's $\tau$ and Pearson's $r$ correlations for BERT-FR-LM with each $k$ on DUC-05.

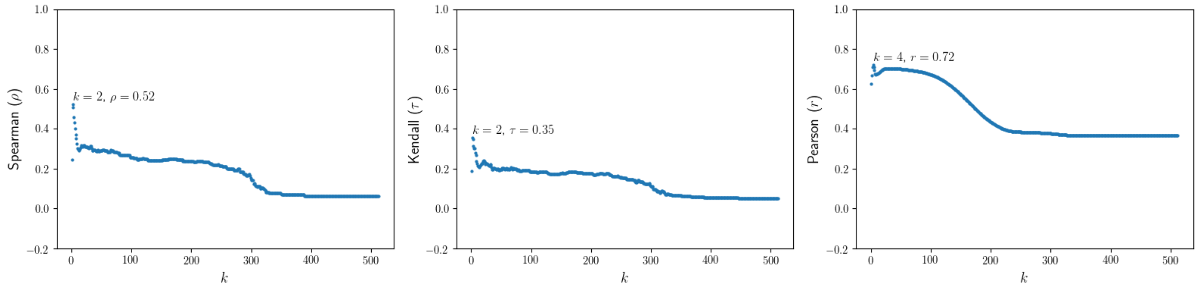


Figure 9: Spearman's $\rho$, Kendall's $\tau$ and Pearson's $r$ correlations for BERT-FR-LM with each $k$ on DUC-06.

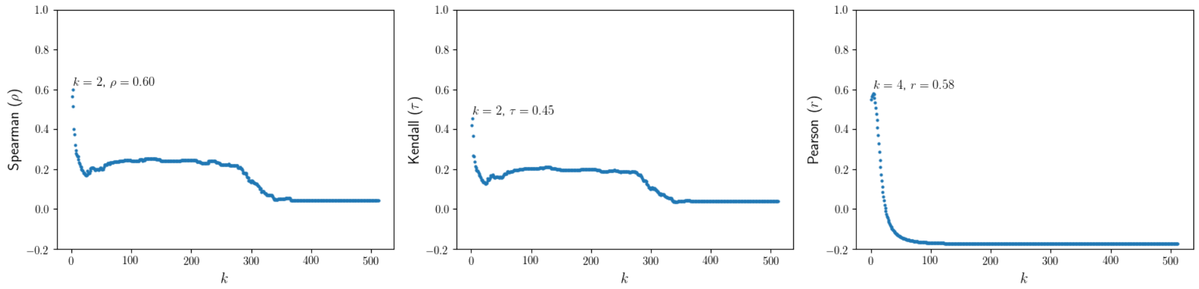


Figure 10: Spearman's $\rho$, Kendall's $\tau$ and Pearson's $r$ correlations for BERT-FR-LM with each $k$ on DUC-07.

"The shift from video disk and CD-ROM to the Internet has also meant that the Library of Congress has been able to shift its potential electronic audience from schools, universities and school libraries to the desk of any person with a computer and modem. The idea then was to duplicate much of the Library of Congress' huge holdings in electronic form so people in other parts of the country could have access to the material without traveling to Washington or even leaving home. This letter and hundreds of others in their original form can be read on the Internet at the American Memory site of the Library of Congress, one of the libraries leading the way in a quiet revolution that is changing the way knowledge is shared around the world. Anyone who wants to pinpoint where James Bond met that blonde with the bottle of champagne on her curvy hip need only consult "Language of the Land," an unusual book published by the Library of Congress offering maps of imaginary places. To spread the word, the Library of Congress has begun a program to show teachers how to use its collection in their classrooms. That the library would grow into a pre-eminent world institution was beyond imagination. The Library of Congress is charged with collecting the creative work of the American people. At last count, the Library of Congress had 9,429,184 books and nearly 110 million other items, in 460 languages."

Figure 11: Example summary from the DUC-07 dataset.

| | $\mathcal{Q}1$ | $\mathcal{Q}2$ | $\mathcal{Q}3$ | $\mathcal{Q}4$ | $\mathcal{Q}5$ |
|---|---|---|---|---|---|
| BiGRU | 4.48 | 5.20 | **3.52** | 3.08 | 1.08 |
| SUM-QE | **4.72** | **4.12** | 2.48 | **3.76** | **2.64** |
| GOLD | 5 | 4 | 4 | 4 | 4 |

Table 1: Scores assigned by SUM-QE and the BiGRU-based baseline to the summary in Figure 11, for all $\mathcal{Q}s$. Comparison to the gold scores available for the summary in the DUC-07 dataset.

## References


Hoa Trang Dang. 2006a. DUC 2005: Evaluation of Question-focused Summarization Systems. In *Proceedings of the Workshop on Task-Focused Summarization and Question Answering*, SumQA '06, pages 48–55, Sydney, Australia.

Hoa Trang Dang. 2006b. Overview of DUC 2006. In *Proceedings of the Document Understanding Workshop at HLT-NAACL 2006*, Brooklyn, NY, USA.

Paul Over, Hoa Dang, and Donna Harman. 2007. DUC in Context. *Information Processing & Management*, 43(6):1506–1520.

Alec Radford, Jeff Wu, Rewon Child, David Luan, Dario Amodei, and Ilya Sutskever. 2019. Language Models are Unsupervised Multitask Learners.
